# Supplementary material for: 3D-LDM: Neural Implicit 3D Shape Generation with Latent Diffusion Models
Source: arXiv:2212.00842 source file (2022-12-15)
Supplement: Supplementary file 1 [file applications.tex]

\begin{figure*}[t]
  \centering
\includegraphics[width=\linewidth,height=0.5\linewidth]{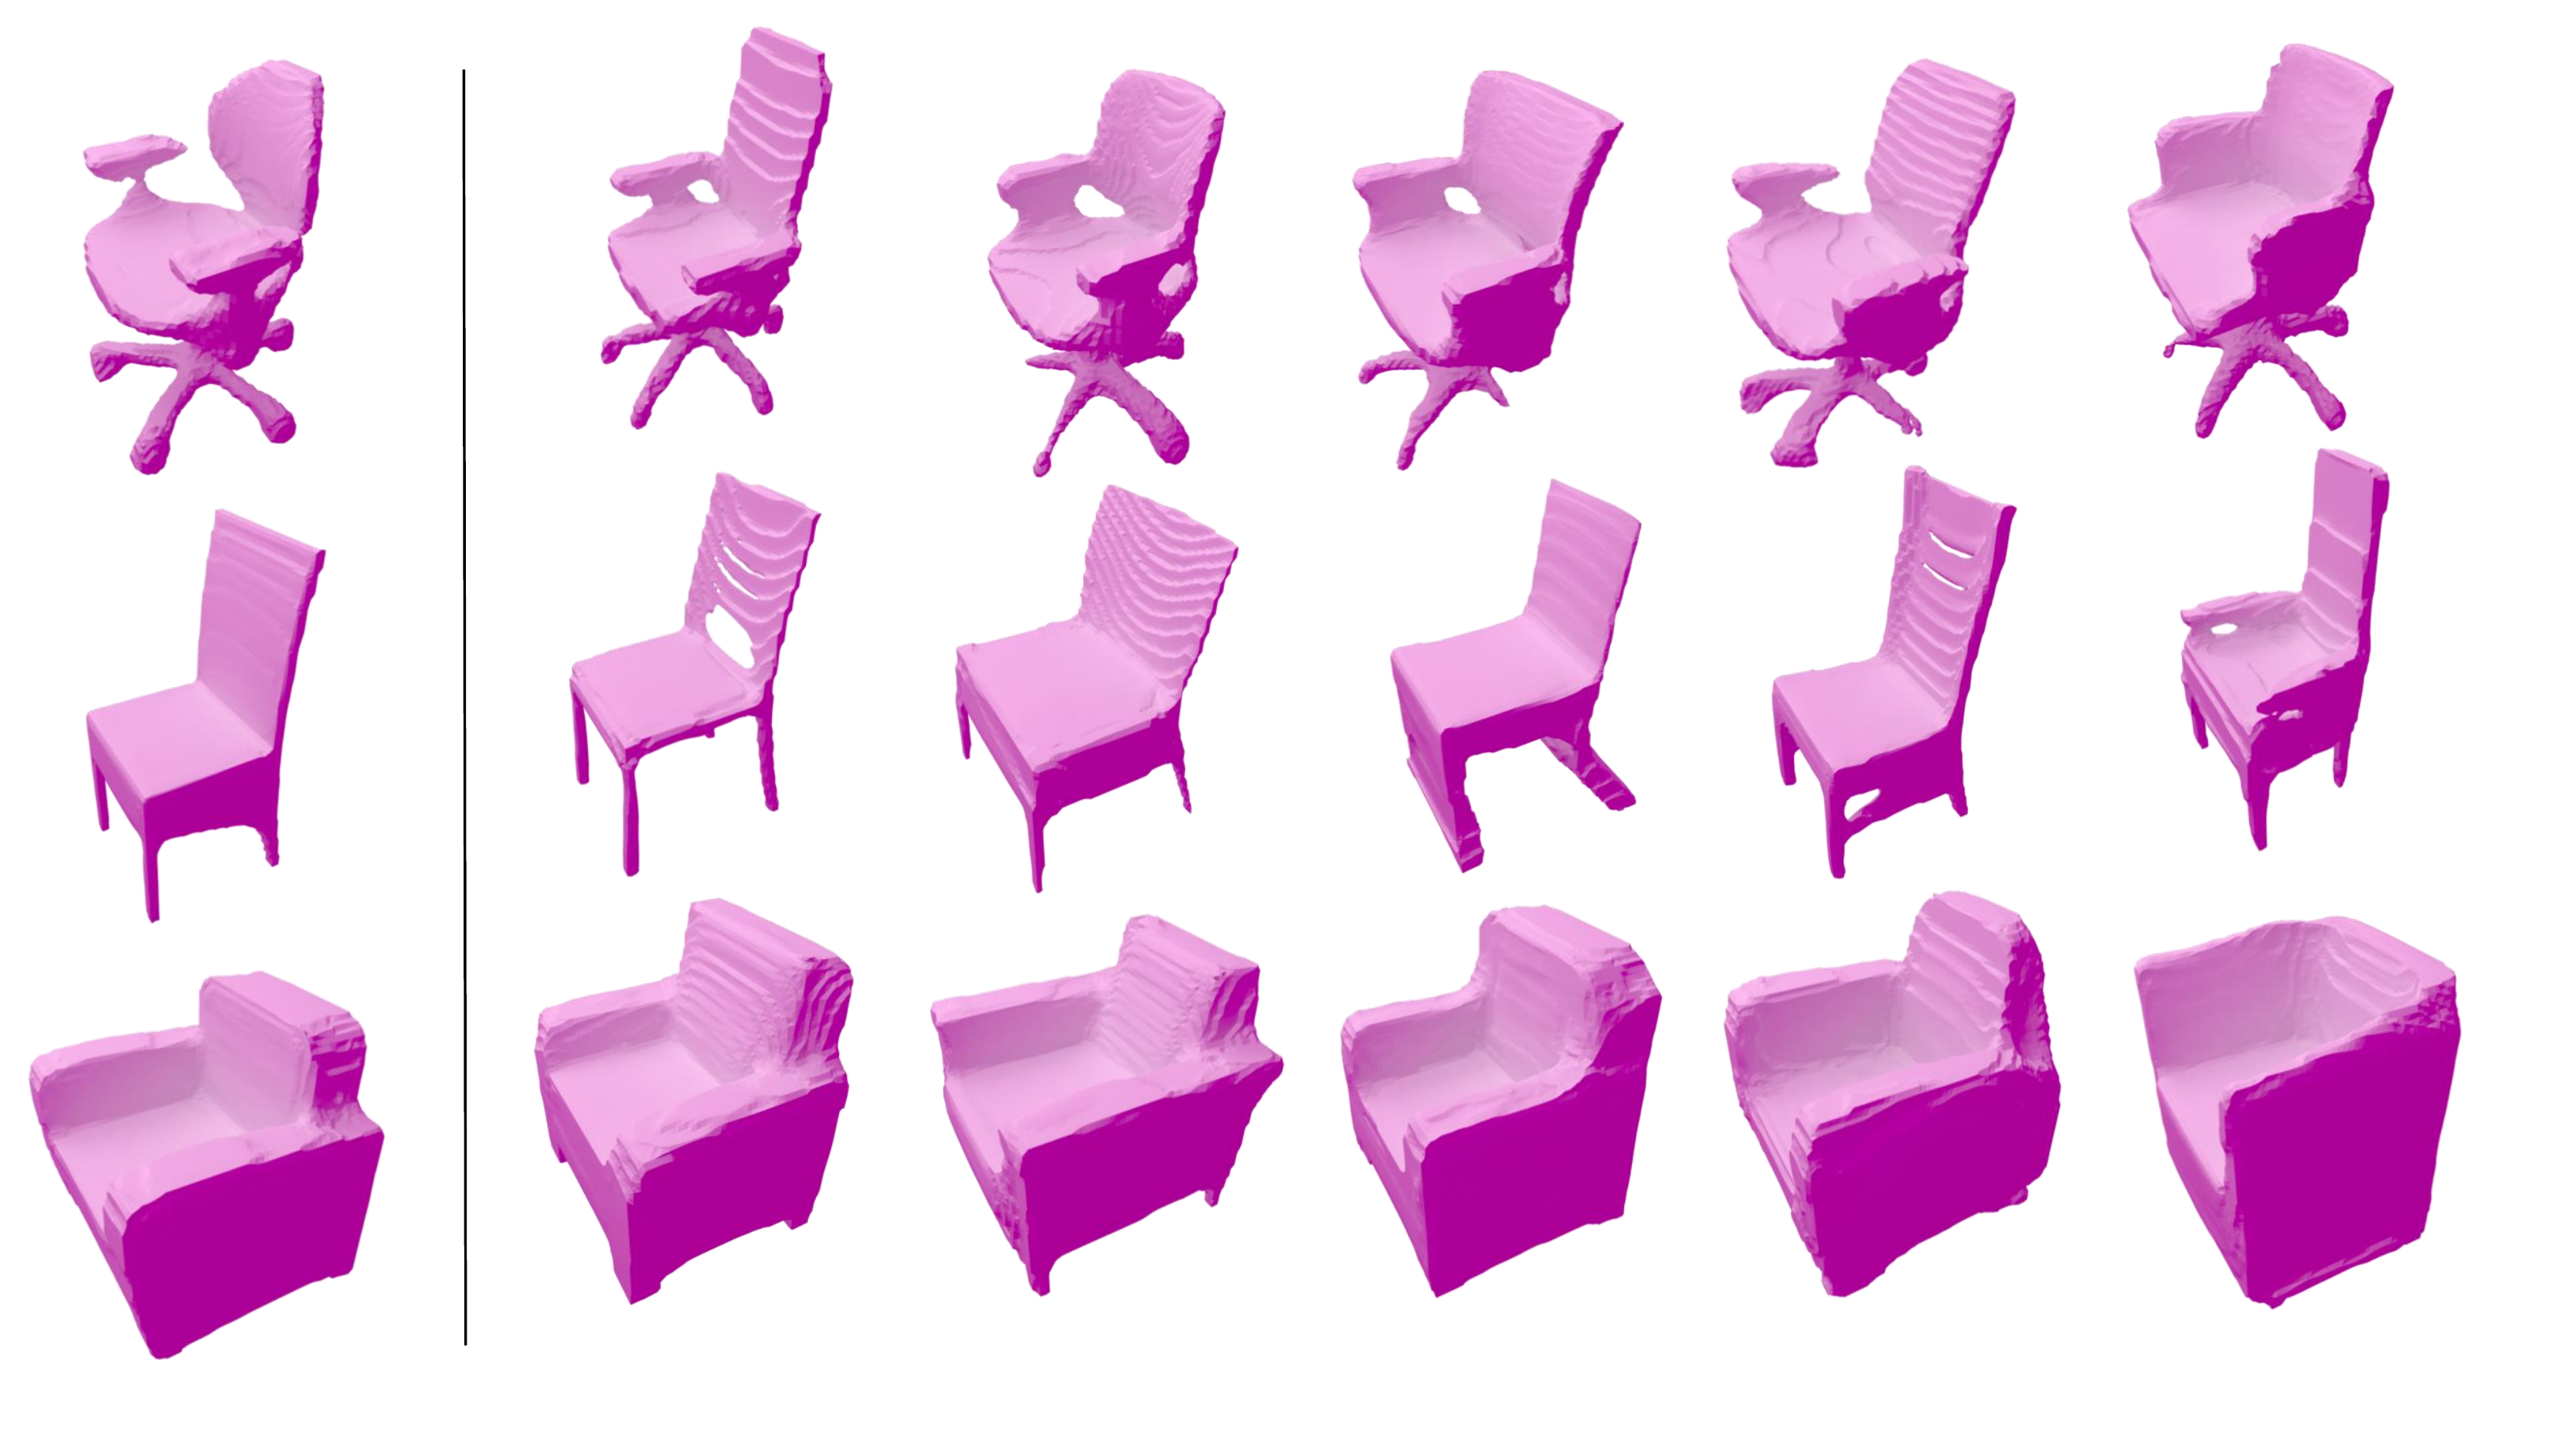}
  \caption{Guided shape exploration. By adding noise to the input shape (left column), we can generate variations of the input shapes that can be used for shape exploration. In each column we show a different generated sample after adding 2000 noise steps to the input shape. We can see that the coarse shape of the input is preserved, but each variation generates different shape detail.}
  \label{fig:exploration}
\end{figure*}

\section{Shape Exploration}
\label{sec:applications}

In this section, we show qualitative results for the shape exploration application mentioned in the main paper. We can explore variations of a given input shape by adding noise to its latent vector and denoising it using our method. The amount of noise controls how similar the generated shape variations are to the input shape. In Figure~\ref{fig:exploration} shows generated variations for three input shapes. The number of noise steps has to be big enough so that the denoising process does not deterministically trace the original shape back and not too big to avoid generating random shapes unrelated to the shape of origin. For our experiments, we add 2000 noise steps and denoise using our method for the same number of steps. We can see that the shape variations explore different shape detail, while preserving the coarse shape of the input.
