# Supplementary material for: 3D-LDM: Neural Implicit 3D Shape Generation with Latent Diffusion Models
Source: arXiv:2212.00842 source file (2022-12-15)
Supplement: Supplementary file 2 [file applications_bis.tex]

\section{CLIP Conditioning}
\label{sec:applications2}

In Figure~\ref{fig:textclip} and Figure~\ref{fig:imclip}, we showcase the versatility of our method by extending it to a conditioning based on CLIP-embeddings~\cite{radford2021learning}. By training a version of \name conditioned on shape renderings encoded through CLIP, we not only allow for shape generation through images which were used for the training part but also text prompts thanks to the common domain  of the text and image embddings in CLIP. For our text-to-shape experiments, we use more descriptive and implicit text such as \textit{"This is a spinning chair with wheels"} instead of the category-based text \textit{"This is an office chair"}. Through the results, we can see that \name conditioned on CLIP embeddings yields reasonable results for both image and text inputs.

\begin{figure}[t]
  \centering
\includegraphics[width=\linewidth]{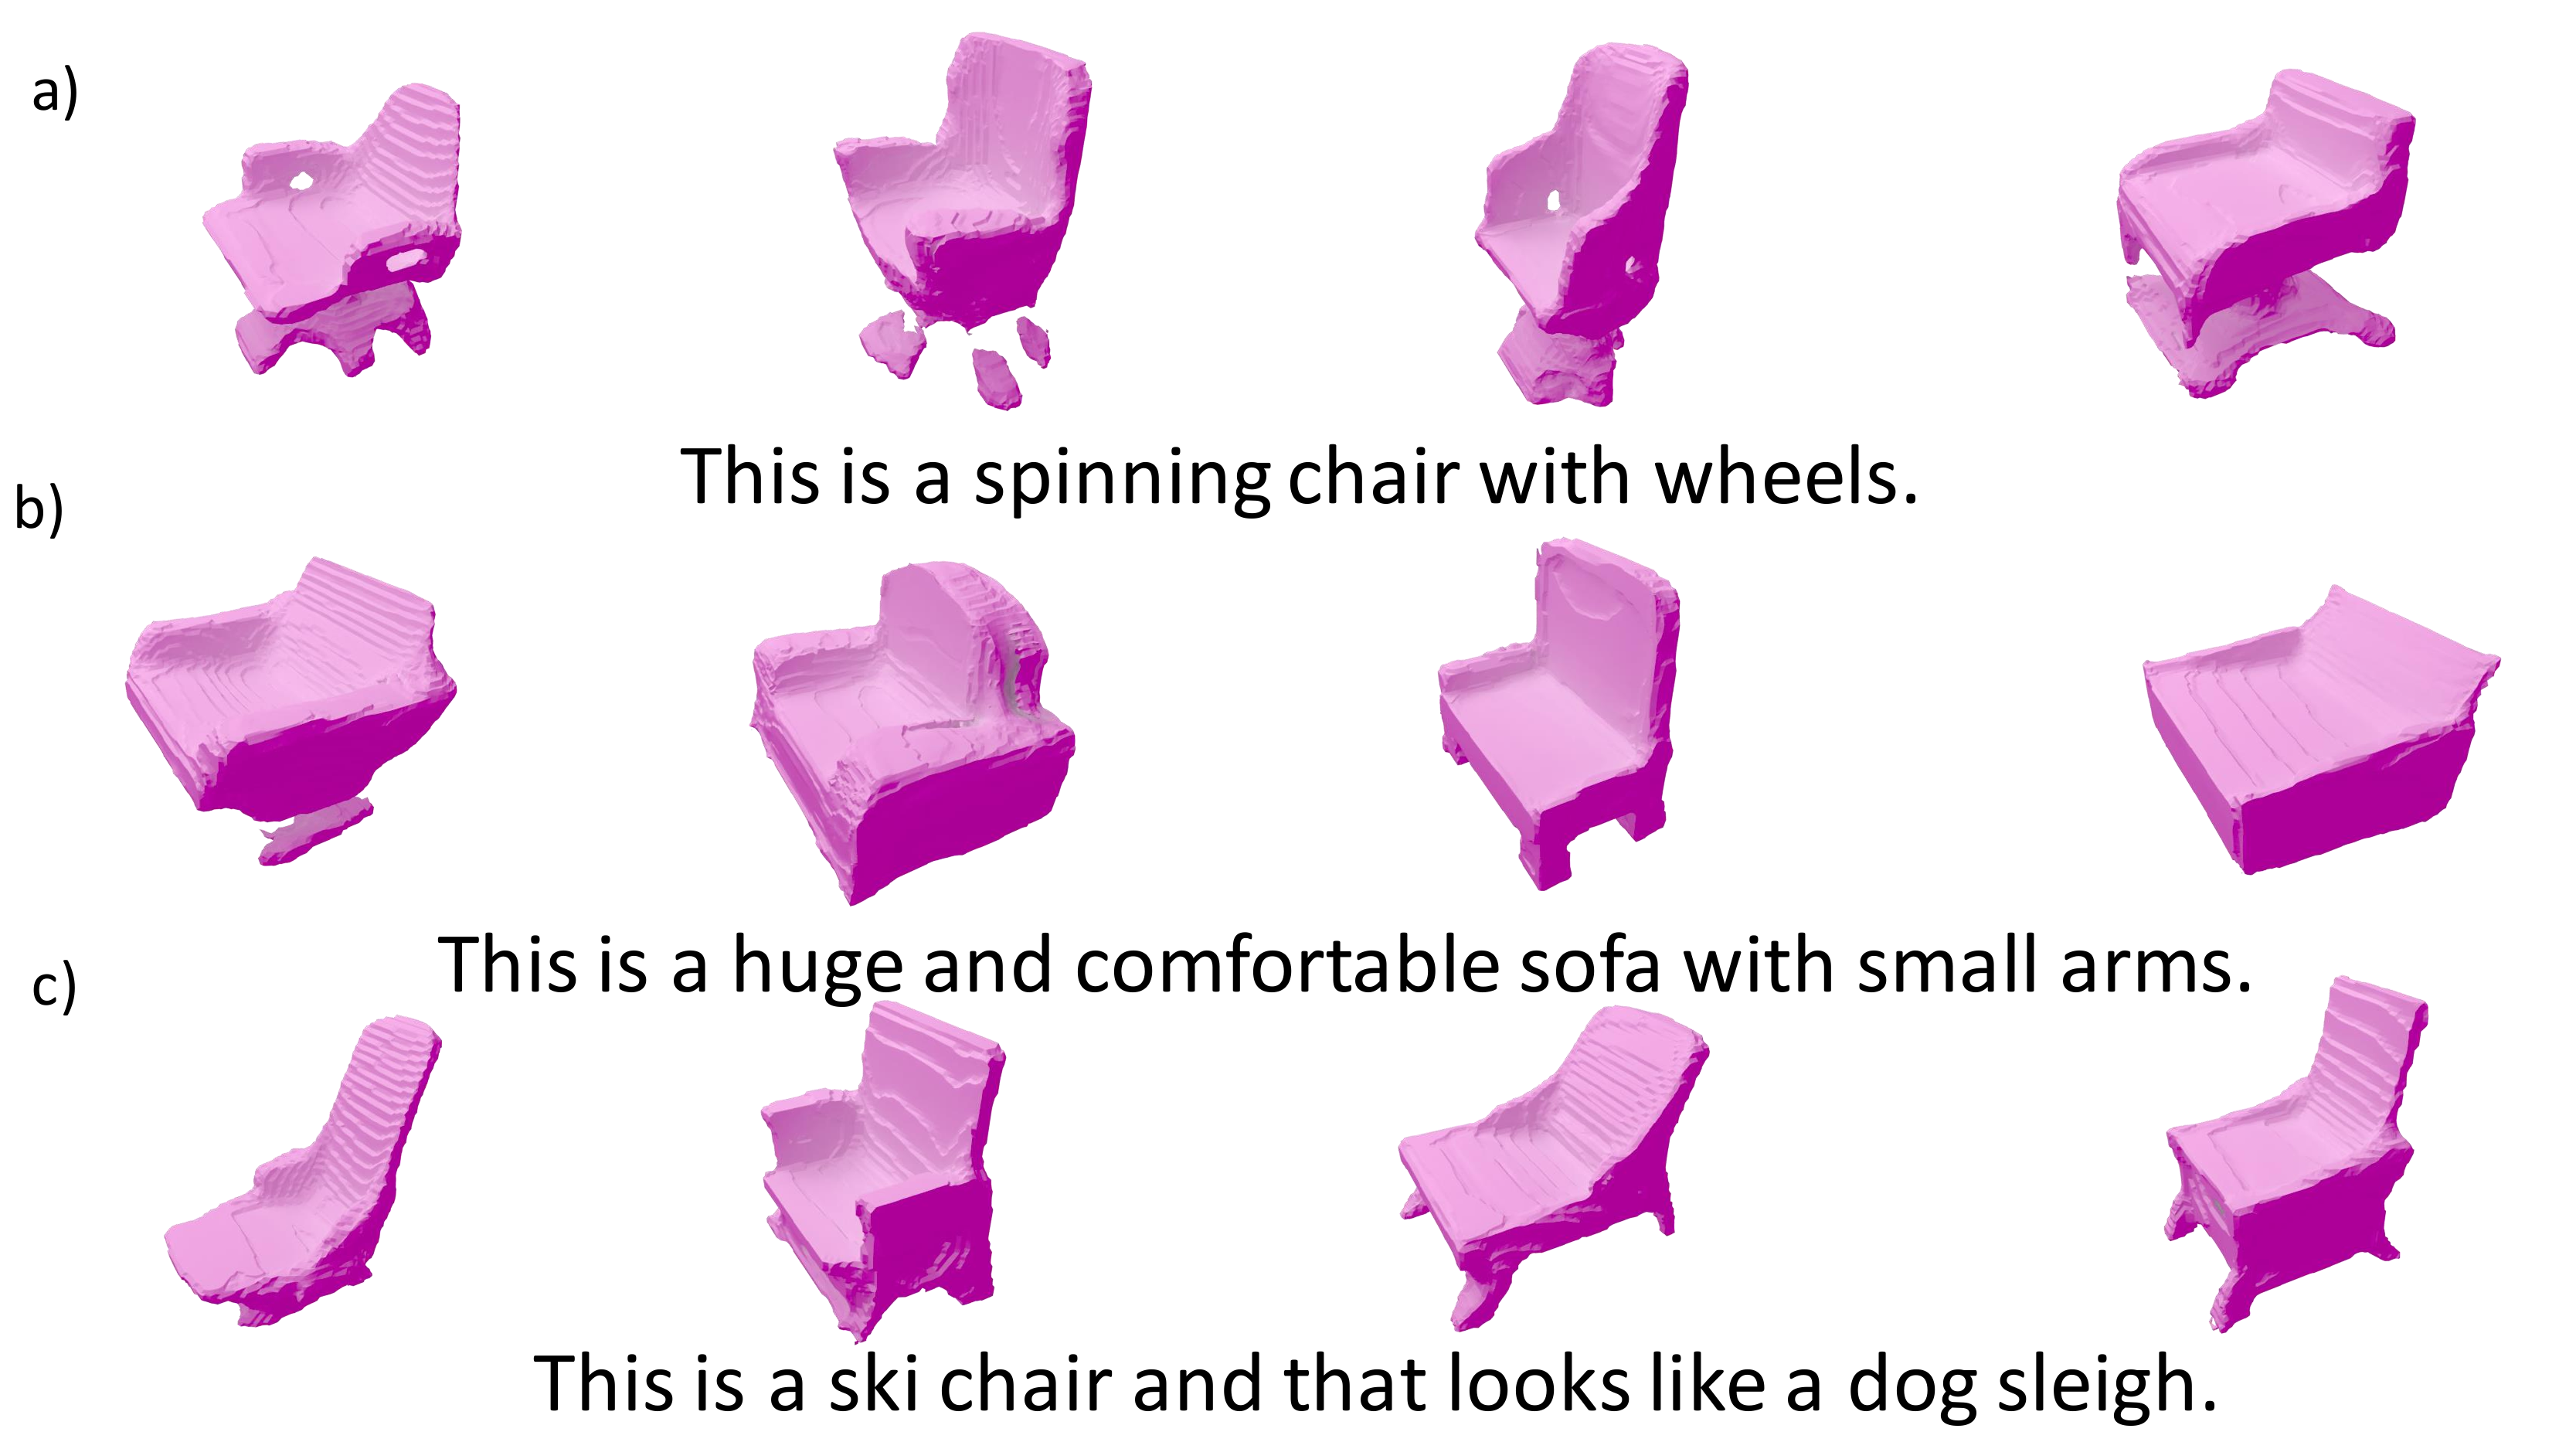}
  \caption{Text-to-Shape. \name conditioned on CLIP embeddings can generate shapes that match the description given by the text prompt. In each row, we showcase multiple shapes generated by our model for each text prompt.}
  \label{fig:textclip}
\end{figure}

\begin{figure}[t]
  \centering
\includegraphics[width=\linewidth]{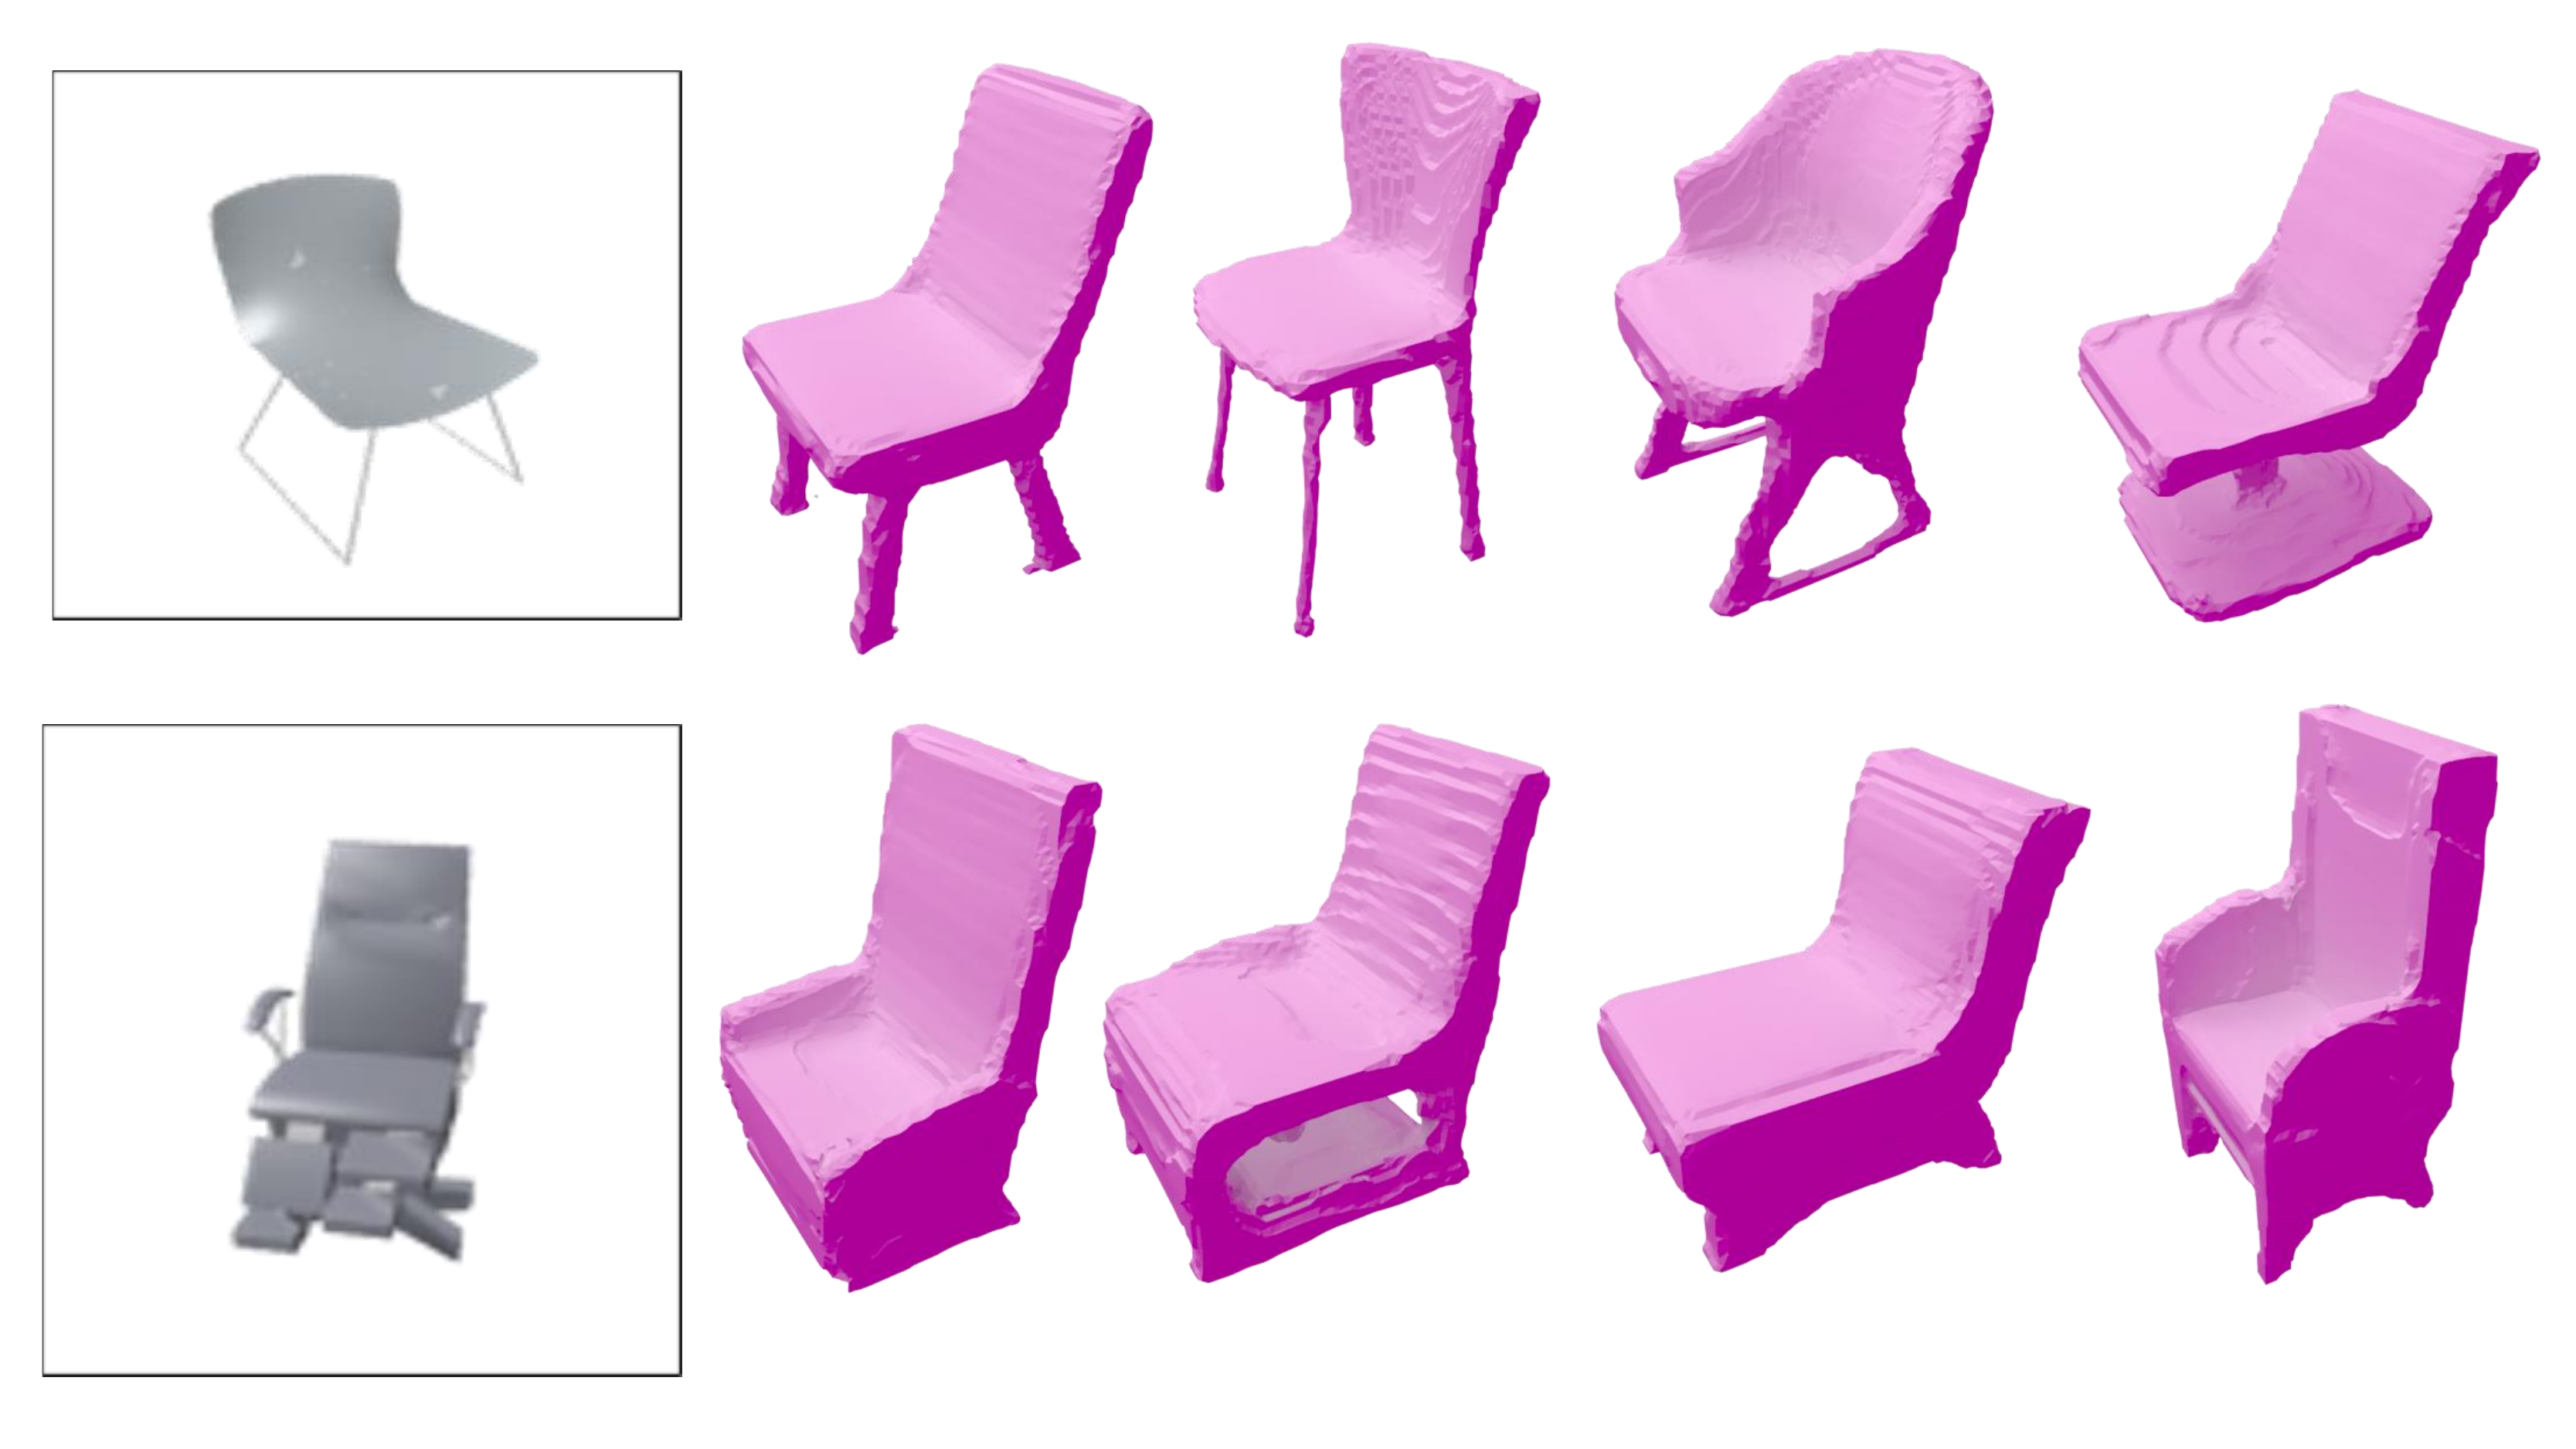}
  \caption{Image-to-Shape. \name conditioned on CLIP embeddings can generate shapes similar to an input image. In each row, we showcase multiple shapes generated by our model for two different image renderings of chairs extracted from the \textit{chairs} dataset.}
  \label{fig:imclip}
\end{figure}
